# Supplementary material for: Optimal Sparse Decision Trees
Source: arXiv:1904.12847 source file (2023-09-26)
Supplement: Supplementary file 1 [file appendix-bounds.tex]

\section{Excessive Antecedent Support}
\label{appendix:ub-supp}

\begin{theorem}[Upper bound on antecedent support]
\label{thm:ub-support}
Let ${\OptimalRL = (\Prefix, \Labels, \Default, K)}$
be any optimal rule list with objective~$\OptimalObj$, \ie
${\OptimalRL \in \argmin_\RL \Obj(\RL, \x, \y)}$,
and let ${\Prefix = (p_1, \dots, p_{k-1},}$
${p_k, \dots, p_K)}$ be its prefix.
For each ${k \le K}$, antecedent~$p_k$ in~$\Prefix$
has support less than or equal to
the fraction of all data not captured by preceding antecedents,
by an amount greater than the regularization parameter~$\Reg$:
\begin{align}
\Supp(p_k, \x \given \Prefix) \le 1 - \Supp(\Prefix^{k-1}, \x) - \Reg,
\label{eq:ub-support}
\end{align}
where ${\Prefix^{k-1} = (p_1, \dots, p_{k-1})}$.
For the last antecedent, \ie when ${p_k = p_K}$, equality implies
that there also exists a shorter optimal rule list
${\RL' = (\Prefix^{K-1}, \Labels', \Default', K - 1) \in}$ ${\argmin_\RL \Obj(\RL, \x, \y)}$.
%with prefix~$\Prefix^{K-1}$.
\end{theorem}

\begin{proof}
First, we focus on the last antecedent~$p_{K+1}$ in a rule list~$\RL'$.
Let ${\RL = (\Prefix, \Labels, \Default, K)}$
be a rule list with prefix ${\Prefix = (p_1, \dots, p_K)}$
and objective ${\Obj(\RL, \x, \y) \ge \OptimalObj}$, where
${\OptimalObj \equiv}$ ${\min_{\RLB} \Obj(\RLB, \x, \y)}$
is the optimal objective.
Let ${\RL' = (\Prefix', \Labels', \Default', K + 1)}$
be a rule list whose prefix ${\Prefix' = (p_1, \dots, p_K, p_{K+1})}$
starts with~$\Prefix$ and ends with a new antecedent~$p_{K+1}$.
Suppose~$p_{K+1}$ in the context of~$\Prefix'$ captures nearly all
data not captured by~$\Prefix$, except for a fraction~$\epsilon$
upper bounded by the regularization parameter~$\Reg$:
\begin{align*}
1 - \Supp(\Prefix, \x) - \Supp(p_{K+1}, \x \given \Prefix') \equiv \epsilon \le \Reg.
\end{align*}
Since~$\Prefix'$ starts with~$\Prefix$,
its prefix misclassification error is at least as great;
the only discrepancy between the misclassification errors
of~$\RL$ and~$\RL'$ can come from the difference between the support of
the set of data not captured by~$\Prefix$ and the support of~$p_{K+1}$:
\begin{align*}
| \Loss(\RL', \x, \y) - \Loss(\RL, \x, \y) | \le
1 - \Supp(\Prefix, \x) - \Supp(p_{K+1}, \x \given \Prefix') = \epsilon.
\end{align*}
The best outcome for~$\RL'$ would occur if its misclassification
error were smaller than that of~$\RL$ by~$\epsilon$, therefore
\begin{align*}
\Obj(\RL', \x, \y) &= \Loss(\RL', \x, \y) + \Reg (K+1) \\
&\ge \Loss(\RL, \x, \y) - \epsilon + \Reg(K+1)
= \Obj(\RL, \x, \y) - \epsilon + \Reg \ge \Obj(\RL, \x, \y) \ge \OptimalObj.
\end{align*}
$\RL'$ is an optimal rule list,
\ie ${\RL' \in \argmin_{\RLB} \Obj(\RLB, \x, y)}$,
if and only if ${\Obj(\RL', \x, \y) = \Obj(\RL, \x, \y) =}$ ${\OptimalObj}$,
which requires ${\epsilon = \Reg}$.
Otherwise, ${\epsilon < \Reg}$, in which case
\begin{align*}
\Obj(\RL', \x, \y) \ge \Obj(\RL, \x, \y) - \epsilon + \Reg
> \Obj(\RL, \x, \y) \ge \OptimalObj,
\end{align*}
therefore $\RL'$ is not optimal, \ie  ${\RL' \notin \argmin_{\RLB} \Obj(\RLB, \x, \y)}$.
This demonstrates the desired result for ${k = K}$.

In the remainder, we prove the bound in~\eqref{eq:ub-support} by contradiction,
in the context of a rule list~$\RL''$.
Let~$\RL$ and~$\RL'$ retain their definitions from above,
thus as before, that the data not captured by~$\Prefix'$
has normalized support~${\epsilon \le \Reg}$, \ie
\begin{align*}
1 - \Supp(\Prefix', \x) = 1 - \Supp(\Prefix, \x) - \Supp(p_{K+1}, \x \given \Prefix') = \epsilon \le \Reg.
\end{align*}
Thus for any rule list~$\RL''$ whose prefix
$\Prefix'' = (p_1, \dots, p_{K+1}, \dots, p_{K'})$ starts
with~$\Prefix'$ and ends with one or more additional rules,
each additional rule~$p_k$ has support
${\Supp(p_k, \x \given \Prefix'') \le}$ ${\epsilon \le \Reg}$,
for all~${k > K+1}$.
By Theorem~\ref{thm:min-capture},
all of the additional rules have insufficient support,
therefore~$\Prefix''$ cannot be optimal,
\ie ${\RL'' \notin \argmin_{\RLB} \Obj(\RLB, \x, \y)}$.
\end{proof}

Similar to Theorem~\ref{thm:min-capture}, our lower bound on
antecedent support, we can apply Theorem~\ref{thm:ub-support}
in the contexts of both constructing rule lists and
rule mining~(\S\ref{sec:setup}).
Theorem~\ref{thm:ub-support} implies that if we only seek a single
optimal rule list, then during branch-and-bound execution,
we can prune a prefix if we ever add an antecedent with support
too similar to the support of the set of data not captured by the
preceding antecedents.
One way to view this result is that if
${\RL = (\Prefix, \Labels, \Default, K)}$
and ${\RL' = (\Prefix', \Labels', \Default', K + 1)}$
are rule lists such that~$\Prefix'$ starts with~$\Prefix$
and ends with an antecedent that captures all or nearly all
data not captured by~$\Prefix$, then the new rule in~$\RL'$
behaves similar to the default rule of~$\RL$.
As a result, the misclassification error of~$\RL'$ must be
similar to that of~$\RL$, and any reduction may not be
sufficient to offset the penalty for longer prefixes.

\begin{proposition}[Excessive antecedent support propagates]
\label{prop:ub-support}
Define~$\StartContains(\Prefix)$ as in~\eqref{eq:start-contains},
and let ${\Prefix = (p_1, \dots, p_{K})}$ be a prefix,
such that its last antecedent~$p_{K}$ has excessive support,
\ie the opposite of the bound in~\eqref{eq:ub-support}:
\begin{align*}
\Supp(p_K, \x \given \Prefix) > 1 - \Supp(\Prefix^{K-1}, \x) - \Reg,
\end{align*}
where ${\Prefix^{K-1} = (p_1, \dots, p_{K-1})}$.
Let ${\RLB = (\PrefixB, \LabelsB, \DefaultB, \kappa)}$
be any rule list with prefix
${\PrefixB =}$ ${(P_1, \dots, P_{\kappa})}$
such that~$\PrefixB$ starts with ${\PrefixB^{K'-1} =}$
${(P_1, \dots, P_{K'-1}) \in \StartContains(\Prefix^{K-1})}$
and~${P_{K'} = p_{K}}$.
It follows that~$P_{K'}$ has excessive support in prefix~$\PrefixB$,
and furthermore, ${\RLB \notin \argmin_{\RL} \Obj(\RL, \x, \y)}$.
\end{proposition}

\begin{proof}
Since ${\PrefixB^{K'} = (P_1, \dots, P_{K'})}$
contains all the antecedents in~$\Prefix$, we have that
\begin{align*}
\Supp(\PrefixB^{K'}, \x) \ge \Supp(\Prefix, \x).
\end{align*}
Expanding these two terms gives
\begin{align*}
\Supp(\PrefixB^{K'}, \x)
&= \Supp(\PrefixB^{K'-1}, \x) + \Supp(P_{K'}, \x \given \PrefixB) \\
&\ge \Supp(\Prefix, \x)
= \Supp(\Prefix^{K-1}, \x) + \Supp(p_K, \x \given \Prefix)
> 1 - \Reg.
\end{align*}
Rearranging gives
\begin{align*}
\Supp(P_{K'}, \x \given \PrefixB)
> 1 - \Supp(\PrefixB^{K'-1}, \x) - \Reg,
\end{align*}
thus~$P_{K'}$ has excessive support in~$\PrefixB$.
By Theorem~\ref{thm:ub-support},
${\RLB \notin \argmin_{\RL} \Obj(\RL, \x, \y)}$.
\end{proof}

\section{Proof of Theorem~\ref{thm:equivalent} (Equivalent Support Bound)}
\label{appendix:equiv-supp}

We begin by defining four related rule lists.
First, let ${\RL = (\Prefix, \Labels, \Default, K)}$
be a rule list with prefix ${\Prefix = (p_1, \dots, p_K)}$
and labels ${\Labels = (q_1, \dots, q_K)}$.
Second, let ${\RLB = (\PrefixB, \LabelsB, \DefaultB, \kappa)}$
be a rule list with prefix ${\PrefixB = (P_1, \dots, P_\kappa)}$
that captures the same data as~$\Prefix$,
and labels ${\LabelsB = (Q_1, \dots, Q_\kappa)}$.
Third, let ${\RL' = (\Prefix', \Labels', \Default', K') \in}$
${\StartsWith(\RL)}$ be any rule list
whose prefix starts with~$\Prefix$, such that~${K' \ge K}$.
Denote the prefix and labels of~$\RL'$ by
${\Prefix' = (p_1, \dots, p_K,}$ ${p_{K+1}, \dots, p_{K'})}$
and ${\Labels = (q_1, \dots, q_{K'})}$, respectively.
Finally, define ${\RLB' = (\PrefixB', \LabelsB', \DefaultB', \kappa') \in}$
${\StartsWith(\PrefixB)}$ to be the `analogous' rule list, \ie whose prefix
${\PrefixB' = (P_1, \dots, P_\kappa, P_{\kappa+1}, \dots, P_{\kappa'}) =}$
${(P_1, \dots, P_\kappa, p_{K+1}, \dots, p_{K'})}$
starts with~$\PrefixB$ and ends with the same ${K'-K}$
antecedents as~$\Prefix'$.
Let ${\LabelsB' = (Q_1, \dots, Q_{\kappa'})}$
denote the labels of~$\RLB'$.

Next, we claim that the difference in the objectives
of rule lists~$\RL'$ and~$\RL$ is the same as the difference
in the objectives of rule lists~$\RLB'$ and~$\RLB$.
Let us expand the first difference as
\begin{align}
&\Obj(\RL', \x, \y) - \Obj(\RL, \x, \y)
  = \Loss(\RL', \x, \y) + \Reg K' - \Loss(\RL, \x, \y) - \Reg K \nn \\
&= \Loss_p(\Prefix', \Labels', \x, \y) + \Loss_0(\Prefix', \Default', \x, \y)
  - \Loss_p(\Prefix, \Labels, \x, \y) - \Loss_0(\Prefix, \Default, \x, \y)
  + \Reg (K' - K). \nn
\end{align}
Similarly, let us expand the second difference as
\begin{align}
&\Obj(\RLB', \x, \y) - \Obj(\RLB, \x, \y)
  = \Loss(\RLB', \x, \y) + \Reg \kappa' - \Loss(\RLB, \x, \y) - \Reg \kappa \nn \\
&= \Loss_p(\PrefixB', \LabelsB', \x, \y) + \Loss_0(\PrefixB', \DefaultB', \x, \y)
  - \Loss_p(\PrefixB, \LabelsB, \x, \y) - \Loss_0(\PrefixB, \DefaultB, \x, \y)
  + \Reg (K' - K), \nn
\end{align}
where we have used the fact that ${\kappa' - \kappa = K' - K}$.

The prefixes~$\Prefix$ and~$\PrefixB$ capture the same data.
Equivalently, the set of data that is not captured by~$\Prefix$
is the same as the set of data that is not captured by~$\PrefixB$, \ie
\begin{align}
\{x_n : \neg\, \Cap(x_n, \Prefix)\} = \{x_n : \neg\, \Cap(x_n, \PrefixB)\}. \nn
\end{align}
Thus, the corresponding rule lists~$\RL$ and~$\RLB$
share the same default rule, \ie ${\Default = \DefaultB}$,
yielding the same default rule misclassification error:
\begin{align}
\Loss_0(\Prefix, \Default, \x, \y) = \Loss_0(\PrefixB, \DefaultB, \x, \y). \nn
\end{align}
Similarly, prefixes~$\Prefix'$ and~$\PrefixB'$ capture
the same data, and thus rule lists~$\RL'$ and~$\RLB'$
have the same default rule misclassification error:
\begin{align}
\Loss_0(\Prefix, \Default, \x, \y) = \Loss_0(\PrefixB, \DefaultB, \x, \y). \nn
\end{align}

At this point, to demonstrate our claim relating the objectives
of~$\RL$, $\RL'$, $\RLB$, and~$\RLB'$, what remains is to
show that the difference in the misclassification errors
of prefixes~$\Prefix'$ and~$\Prefix$ is the same as that
between~$\PrefixB'$ and~$\PrefixB$.
We can expand the first difference as
\begin{align}
\Loss_p(\Prefix', \Labels', \x, \y) - \Loss_p(\Prefix, \Labels, \x, \y)
%&= \frac{1}{N} \sum_{n=1}^N \sum_{k=1}^{K'}
%  \one [ \Cap(x_n, p_k \given \Prefix') \wedge (q_k \neq y_n) ]
%  - \frac{1}{N} \sum_{n=1}^N \sum_{k=1}^K
%  \one [ \Cap(x_n, p_k \given \Prefix) \wedge (q_k \neq y_n) ] \\
&= \frac{1}{N} \sum_{n=1}^N \sum_{k=K+1}^{K'}
  \Cap(x_n, p_k \given \Prefix') \wedge \one [ q_k \neq y_n ], \nn
\end{align}
where we have used the fact that since~$\Prefix'$
starts with~$\Prefix$, the first~$K$ rules in~$\Prefix'$
make the same mistakes as those in~$\Prefix$.
Similarly, we can expand the second difference as
\begin{align}
\Loss_p(\PrefixB', \LabelsB', \x, \y) - \Loss_p(\PrefixB, \LabelsB, \x, \y)
&= \frac{1}{N} \sum_{n=1}^N \sum_{k=\kappa+1}^{\kappa'}
  \Cap(x_n, P_k \given \PrefixB') \wedge \one [ Q_k \neq y_n ] \nn \\
&= \frac{1}{N} \sum_{n=1}^N \sum_{k=K+1}^{K'}
  \Cap(x_n, p_k \given \PrefixB') \wedge \one [ Q_k \neq y_n ] \nn \\
&= \frac{1}{N} \sum_{n=1}^N \sum_{k=K+1}^{K'}
  \Cap(x_n, p_k \given \Prefix') \wedge \one [ q_k \neq y_n ] \label{eq:third} \\
&= \Loss_p(\Prefix', \Labels', \x, \y) - \Loss_p(\Prefix, \Labels, \x, \y) \nn.
\end{align}
To justify the equality in~\eqref{eq:third}, we observe first that
prefixes~$\PrefixB'$ and~$\Prefix'$ start with~$\kappa$ and~$K$
antecedents, respectively, that capture the same data.
Second, prefixes~$\PrefixB'$ and~$\Prefix'$ end with exactly
the same ordered list of~${K' - K}$ antecedents,
therefore for any~${k = 1, \dots, K' - K}$,
antecedent ${P_{\kappa + k} = p_{K + k}}$ in~$\PrefixB'$
captures the same data as~$p_{K + k}$ captures in~$\Prefix'$.
It follows that the corresponding labels are all equivalent, \ie
${Q_{\kappa + k} = q_{K + k}}$, for all~${k = 1, \dots, K' - K}$,
and consequently, the prefix misclassification error associated
with the last~${K' - K}$ antecedents of~$\Prefix'$ is the same
as that of~$\PrefixB'$.
We have therefore shown that the difference between the objectives
of~$\RL'$ and~$\RL$ is the same as that between~$\RLB'$ and~$\RLB$, \ie
\begin{align}
\Obj(\RL', \x, \y) - \Obj(\RL, \x, \y)
= \Obj(\RLB', \x, \y) - \Obj(\RLB, \x, \y).
\label{eq:equiv-analogous}
\end{align}

Next, suppose that the objective lower bounds of~$\RL$ and~$\RLB$
obey ${b(\Prefix, \x, \y) \le b(\PrefixB, \x, \y)}$, therefore
\begin{align}
\Obj(\RL, \x, \y)
&= \Loss_p(\Prefix, \Labels, \x, \y) + \Loss_0(\Prefix, \Default, \x, \y) + \Reg K \nn \\
&= b(\Prefix, \x, \y) + \Loss_0(\Prefix, \Default, \x, \y) \nn \\
&\le b(\PrefixB, \x, \y) + \Loss_0(\Prefix, \Default, \x, \y)
= b(\PrefixB, \x, \y) + \Loss_0(\PrefixB, \DefaultB, \x, \y)
= \Obj(\RLB, \x, \y).
\label{eq:equiv-ineq}
\end{align}
Now let~$\RL^*$ be an optimal rule list with prefix
constrained to start with~$\Prefix$,
\begin{align}
\RL^* \in \argmin_{\RL^\dagger \in \StartsWith(\RL)} \Obj(\RL^\dagger, \x, \y), \nn
\end{align}
and let~$K^*$ be the length of~$\RL^*$.
Let~$\RLB^*$ be the analogous $\kappa^*$-rule list whose prefix starts
with~$\PrefixB$ and ends with the same~${K^* - K}$ antecedents as~$\RL^*$,
where~${\kappa^* = \kappa + K^* - K}$.
By~\eqref{eq:equiv-analogous},
\begin{align}
\Obj(\RL^*, \x, \y) - \Obj(\RL, \x, \y)
= \Obj(\RLB^*, \x, \y) - \Obj(\RLB, \x, \y).
\label{eq:equiv-diff}
\end{align}
Furthermore, we claim that~$\RLB^*$ is an optimal rule list
with prefix constrained to start with~$\PrefixB$,
\begin{align}
\RLB^* \in \argmin_{\RLB^\dagger \in \StartsWith(\PrefixB)} \Obj(\RLB^\dagger, \x, \y).
\label{eq:equiv-analogous-optimal}
\end{align}

To demonstrate~\eqref{eq:equiv-analogous-optimal},
we consider two separate scenarios.
In the first scenario, prefixes~$\Prefix$ and~$\PrefixB$
are composed of the same antecedents,
\ie the two prefixes are equivalent up to a permutation of
their antecedents, and as a consequence,
${\kappa = K}$ and~${\kappa^* = K^*}$.
Here, every rule list~${\RL'' \in \StartsWith(\RL)}$
that starts with~$\Prefix$
has an analogue~${\RLB'' \in \StartsWith(\PrefixB)}$
that starts with~$\PrefixB$,
such that~$\RL''$ and~$\RLB''$ obey~\eqref{eq:equiv-analogous},
and vice versa, and thus~\eqref{eq:equiv-analogous-optimal}
is a direct consequence of~\eqref{eq:equiv-diff}.

In the second scenario, prefixes~$\Prefix$ and~$\PrefixB$
are not composed of the same antecedents.
Define~${\phi = \{p_k : (p_k \in \Prefix) \wedge (p_k \notin \PrefixB)\}}$
to be the set of antecedents in~$\Prefix$ that are not in~$\PrefixB$,
and define~${\Phi = \{P_k : (P_k \in \PrefixB) \wedge (P_k \notin \Prefix)\}}$
to be the set of antecedents in~$\PrefixB$ that are not in~$\Prefix$;
either~${\phi \neq \emptyset}$, or~${\Phi \neq \emptyset}$, or both.

Suppose~${\phi \neq \emptyset}$, and let~${p \in \phi}$
be an antecedent in~$\phi$.
It follows that there exists a subset of rule lists
in~$\StartsWith(\PrefixB)$ that do not have analogues
in~$\StartsWith(\RL)$.
Let~${\RLB'' \in \StartsWith(\PrefixB)}$ be such a rule list,
such that its prefix ${\PrefixB'' = (P_1, \dots, P_\kappa, \dots, p, \dots)}$
starts with~$\PrefixB$ and contains~$p$ among its remaining antecedents.
Since~$p$ captures a subset of the data that~$\Prefix$ captures,
and~$\PrefixB$ captures the same data as~$\Prefix$,
it follows that~$p$ does not capture any data in~$\PrefixB''$, \ie
\begin{align}
\frac{1}{N} \sum_{n=1}^N \Cap(x_n, p \given \PrefixB'') = 0 \le \Reg. \nn
\end{align}
By Theorem~\ref{thm:min-capture}, antecedent~$p$ has insufficient
support in~$\RLB''$, and thus~$\RLB''$ cannot be optimal, \ie
${\RLB'' \notin}$ ${\argmin_{\RLB^\dagger \in \StartsWith(\PrefixB)} \Obj(\RLB^\dagger, \x, \y)}$.
By a similar argument, if~${\Phi \neq \emptyset}$
and~${P \in \Phi}$, and~${\RL'' \in \StartsWith(\RL)}$
is any rule list whose prefix starts with~$\Prefix$
and contains antecedent~$P$, then~$\RL''$ cannot be optimal, \ie
${\RL'' \notin \argmin_{\RL^\dagger \in \StartsWith(\RL)} \Obj(\RL^\dagger, \x, \y)}$.

To finish justifying claim~\eqref{eq:equiv-analogous-optimal}
for the second scenario, first define
\begin{align}
\tau(\Prefix, \Phi) \equiv
  \{\RL'' = (\Prefix'', \Labels'', \Default'', K'') :
    \RL'' \in \StartsWith(\RL) \textnormal{ and }
    p_k \notin \Phi, \forall p_k \in \Prefix''\} \subset \StartsWith(\RL) \nn
\end{align}
to be the set of all rule lists whose prefixes start with~$\Prefix$
and do not contain any antecedents in~$\Phi$.
Now, recognize that the optimal prefixes in~$\tau(\Prefix, \Phi)$
and~$\StartsWith(\RL)$ are the same, \ie
\begin{align}
\argmin_{\RL^\dagger \in \tau(\Prefix, \Phi)} \Obj(\RL^\dagger, \x, \y)
= \argmin_{\RL^\dagger \in \StartsWith(\RL)} \Obj(\RL^\dagger, \x, \y), \nn
\end{align}
and similarly, the optimal prefixes in~$\tau(\PrefixB, \phi)$
and~$\StartsWith(\PrefixB)$ are the same, \ie
\begin{align}
\argmin_{\RLB^\dagger \in \tau(\PrefixB, \phi)} \Obj(\RLB^\dagger, \x, \y)
= \argmin_{\RLB^\dagger \in \StartsWith(\PrefixB)} \Obj(\RLB^\dagger, \x, \y). \nn
\end{align}
Since we have shown that every~${\RL'' \in \tau(\Prefix, \Phi)}$
has a direct analogue~${\RLB'' \in \tau(\PrefixB, \phi)}$,
such that~$\RL''$ and~$\RLB''$ obey~\eqref{eq:equiv-analogous},
and vice versa, we again have~\eqref{eq:equiv-analogous-optimal}
as a consequence of~\eqref{eq:equiv-diff}.

We can now finally combine~\eqref{eq:equiv-ineq}
and~\eqref{eq:equiv-analogous-optimal} to obtain the desired inequality in~\eqref{eq:equivalent}:
\begin{align}
\min_{\RL' \in \StartsWith(\RL)} \Obj(\RL', \x, \y)
= \Obj(\RL^*, \x, \y) \le \Obj(\RLB^*, \x, \y)
= \min_{\RLB' \in \StartsWith(\PrefixB)} \Obj(\RLB', \x, \y). \nn
\end{align}

%\clearpage
\section{Proof of Theorem~\ref{thm:similar} (Similar Support Bound)}
\label{appendix:similar-supp}

We begin by defining four related rule lists.
First, let ${\RL = (\Prefix, \Labels, \Default, K)}$
be a rule list with prefix ${\Prefix = (p_1, \dots, p_K)}$
and labels ${\Labels = (q_1, \dots, q_K)}$.
Second, let ${\RLB = (\PrefixB, \LabelsB, \DefaultB, \kappa)}$
be a rule list with prefix ${\PrefixB = (P_1, \dots, P_\kappa)}$
and labels ${\LabelsB = (Q_1, \dots, Q_\kappa)}$.
Define~$\omega$ as in~\eqref{eq:omega}
and~$\Omega$ as in~\eqref{eq:big-omega},
and require that~${\omega, \Omega \le \Reg}$.
Third, let ${\RL' = (\Prefix', \Labels', \Default', K') \in}$
${\StartsWith(\RL)}$ be any rule list
whose prefix starts with~$\Prefix$, such that~${K' \ge K}$.
Denote the prefix and labels of~$\RL'$ by
${\Prefix' = (p_1, \dots, p_K, p_{K+1}, \dots, p_{K'})}$
and ${\Labels = (q_1, \dots, q_{K'})}$,
respectively.
Finally, define
${\RLB' = (\PrefixB', \LabelsB', \DefaultB', \kappa') \in \StartsWith(\PrefixB)}$
to be the `analogous' rule list, \ie whose prefix
${\PrefixB' =}$ ${(P_1, \dots, P_\kappa, P_{\kappa+1}, \dots, P_{\kappa'})
= (P_1, \dots, P_\kappa, p_{K+1}, \dots, p_{K'})}$
starts with~$\PrefixB$ and ends with the same ${K'-K}$
antecedents as~$\Prefix'$.
Let ${\LabelsB' = (Q_1, \dots, Q_{\kappa'})}$
denote the labels of~$\RLB'$.

%Suppose that the lower bounds of~$\Prefix$ and~$\PrefixB$
%obey ${b(\Prefix, \x, \y) < b(\PrefixB, \x, \y)}$.
%
The smallest possible objective for~$\RLB'$, in relation
to the objective of~$\RL'$, reflects both the difference
between the objective lower bounds of~$\RLB$ and~$\RL$
and the largest possible discrepancy between the
objectives of~$\RL'$ and~$\RLB'$.
The latter would occur if~$\RL'$ misclassified all the data
corresponding to both~$\omega$ and~$\Omega$ while~$\RLB'$
correctly classified this same data, thus
\begin{align}
\Obj(\RLB', \x, \y) \ge \Obj(\RL', \x, \y)
  + b(\PrefixB, \x, \y) - b(\Prefix, \x, \y) - \omega - \Omega.
\label{eq:similar-analogous}
\end{align}
Now let~$\RLB^*$ be an optimal rule list with prefix
constrained to start with~$\PrefixB$,
\begin{align*}
\RLB^* \in \argmin_{\RLB^\dagger \in \StartsWith(\PrefixB)} \Obj(\RLB^\dagger, \x, \y),
\end{align*}
and let~$\kappa^*$ be the length of~$\RLB^*$.
Also let~$\RL^*$ be the analogous $K^*$-rule list whose prefix
starts with~$\Prefix$ and ends with the same~${\kappa^* - \kappa}$
antecedents as~$\RLB^*$, where~${K^* = K + \kappa^* - \kappa}$.
By~\eqref{eq:similar-analogous}, we obtain the desired inequality in~\eqref{eq:similar}:
\begin{align*}
\min_{\RLB^\dagger \in \StartsWith(\PrefixB)} \Obj(\RLB^\dagger, \x, \y)
&= \Obj(\RLB^*, \x, \y) \\
&\ge \Obj(\RL^*, \x, \y)
  + b(\PrefixB, \x, \y) - b(\Prefix, \x, \y) - \omega - \Omega \\
&\ge \min_{\RL^\dagger \in \StartsWith(\RL)} \Obj(\RL^\dagger, \x, \y)
  + b(\PrefixB, \x, \y) - b(\Prefix, \x, \y) - \omega - \Omega.
\end{align*}

\section{Proof of Theorem~\ref{thm:identical} (Equivalent Points Bound)}
\label{appendix:equiv-pts}

We derive a lower bound on the default rule
misclassification error~$\Loss_0(\Prefix, \Default, \x, \y)$,
analogous to the lower bound~\eqref{eq:lb-equiv-pts} on the misclassification
error~$\Loss(\RL, \x, \y)$ in the proof of Proposition~\ref{prop:identical}.
As before, we sum over all sets of equivalent points, and then for each such set,
we count differences between class labels and the minority class label of the set,
instead of counting mistakes made by the default rule:
\begin{align}
\Loss_0(\Prefix, \Default, \x, \y)
&= \frac{1}{N} \sum_{n=1}^N \neg\, \Cap(x_n, \Prefix) \wedge \one [ q_0 \neq y_n ] \nn \\
&= \frac{1}{N} \sum_{u=1}^U \sum_{n=1}^N \neg\, \Cap(x_n, \Prefix) \wedge
  \one [ q_0 \neq y_n ]\, \one [ x_n \in e_u ] \nn \\
&\ge \frac{1}{N} \sum_{u=1}^U \sum_{n=1}^N \neg\, \Cap(x_n, \Prefix) \wedge
  \one [ y_n = q_u ]\, \one [ x_n \in e_u ] = b_0(\Prefix, \x, \y),
\label{eq:lb-equiv-pts-uncap}
\end{align}
where the final equality comes from the definition of~$b_0(\Prefix, \x, \y)$ in~\eqref{eq:lb-b0}.
Since we can write the objective~$\Obj(\RL, \x, \y)$
as the sum of the objective lower bound~$b(\Prefix, \x, \y)$ and
default rule misclassification error~$\Loss_0(\Prefix, \Default, \x, \y)$,
applying~\eqref{eq:lb-equiv-pts-uncap} gives a lower bound on~$\Obj(\RL, \x, \y)$:
\begin{align}
\Obj(\RL, \x, \y)
= \Loss_p(\Prefix, \Labels, \x, \y) + \Loss_0(\Prefix, \Default, \x, \y) + \Reg K
&= b(\Prefix, \x, \y) + \Loss_0(\Prefix, \Default, \x, \y) \nn \\
&\ge b(\Prefix, \x, \y) + b_0(\Prefix, \x, \y).
\label{eq:equiv-pts-base}
\end{align}
It follows that for any rule list~${\RL' \in \StartsWith(\RL)}$ whose prefix~$\Prefix'$
starts with~$\Prefix$, we have
\begin{align}
\Obj(\RL', \x, \y) \ge b(\Prefix', \x, \y) + b_0(\Prefix', \x, \y).
\label{eq:equiv-pts-extend}
\end{align}

Finally, we show that the lower bound
on~${\Obj(\RL, \x, \y)}$ in~\eqref{eq:equiv-pts-base} is not greater than
the lower bound on~${\Obj(\RL', \x, \y)}$ in~\eqref{eq:equiv-pts-extend}.
First, let us define
\begin{align}
\Upsilon(\Prefix', K, \x, \y) \equiv \frac{1}{N} \sum_{u=1}^U \sum_{n=1}^N
    \sum_{k=K+1}^{K'} \Cap(x_n, p_k \given \Prefix') \wedge \one [ x_n \in e_u ]\, \one [ y_n = q_u ].
\label{eq:upsilon}
\end{align}
Now, we write a lower bound on~${b(\Prefix', \x, \y)}$ with respect to~${b(\Prefix, \x, \y)}$:
\begin{align}
&b(\Prefix', \x, \y) = \Loss_p(\Prefix', \Labels, \x, \y) + \Reg K'
= \frac{1}{N} \sum_{n=1}^N \sum_{k=1}^{K'} \Cap(x_n, p_k \given \Prefix') \wedge \one [ q_k \neq y_n ] + \Reg K' \nn \\
&= \Loss_p(\Prefix, \Labels, \x, \y) + \Reg K + \frac{1}{N} \sum_{n=1}^N \sum_{k=K}^{K'} \Cap(x_n, p_k \given \Prefix') \wedge \one [ q_k \neq y_n ] + \Reg (K' - K) \nn \\
&= b(\Prefix, \x, \y) + \frac{1}{N} \sum_{n=1}^N \sum_{k=K+1}^{K'} \Cap(x_n, p_k \given \Prefix') \wedge \one [ q_k \neq y_n ] + \Reg (K' - K) \nn \\
&= b(\Prefix, \x, \y) + \frac{1}{N} \sum_{u=1}^U \sum_{n=1}^N \sum_{k=K+1}^{K'} \Cap(x_n, p_k \given \Prefix')
  \wedge \one [ q_k \neq y_n ]\, \one [ x_n \in e_u ] + \Reg (K' - K) \nn \\
&\ge b(\Prefix, \x, \y) + \frac{1}{N} \sum_{u=1}^U \sum_{n=1}^N \sum_{k=K+1}^{K'} \Cap(x_n, p_k \given \Prefix')
  \wedge \one [ y_n = q_u ]\, \one [ x_n \in e_u ] + \Reg (K' - K) \nn \\
&= b(\Prefix, \x, \y) + \Upsilon(\Prefix', K, \x, \y) + \Reg (K' - K),
\label{eq:equiv-pts-b}
\end{align}
where the last equality uses~\eqref{eq:upsilon}.
Next, we write ${b_0(\Prefix, \x, \y)}$ with respect to~${b_0(\Prefix', \x, \y)}$,
\begin{align}
&b_0(\Prefix, \x, \y) = \frac{1}{N} \sum_{u=1}^U \sum_{n=1}^N
    \neg\, \Cap(x_n, \Prefix) \wedge \one [ x_n \in e_u ]\, \one [ y_n = q_u ] \nn \\
&= \frac{1}{N} \sum_{u=1}^U \sum_{n=1}^N
    \left(\neg\, \Cap(x_n, \Prefix')+ \sum_{k=K+1}^{K'} \Cap(x_n, p_k \given \Prefix') \right)
    \wedge \one [ x_n \in e_u ]\, \one [ y_n = q_u ] \nn \\
&= b_0(\Prefix', \x, \y) + \frac{1}{N} \sum_{u=1}^U \sum_{n=1}^N
    \sum_{k=K+1}^{K'} \Cap(x_n, p_k \given \Prefix') \wedge \one [ x_n \in e_u ]\, \one [ y_n = q_u ].
\label{eq:b0}
\end{align}
Rearranging~\eqref{eq:b0} gives
\begin{align}
b_0(\Prefix', \x, \y) &= b_0(\Prefix, \x, y) - \Upsilon(\Prefix', K, \x, \y).
\label{eq:equiv-pts-b0}
\end{align}
Combining~\eqref{eq:equiv-pts-extend} with first~\eqref{eq:equiv-pts-b0}
and then~\eqref{eq:equiv-pts-b} gives the desired inequality in~\eqref{eq:identical}:
\begin{align}
\Obj(\RL', \x, \y) &\ge b(\Prefix', \x, \y) + b_0(\Prefix', \x, \y) \nn \\
&= b(\Prefix', \x, \y) + b_0(\Prefix, \x, y) - \Upsilon(\Prefix', K, \x, \y) \nn \\
&\ge b(\Prefix, \x, \y) + \Upsilon(\Prefix', K, \x, \y) + \Reg (K' - K) + b_0(\Prefix, \x, y) - \Upsilon(\Prefix', K, \x, \y) \nn \\
&= b(\Prefix, \x, \y) + b_0(\Prefix, \x, y) + \Reg (K' - K)
\ge b(\Prefix, \x, \y) + b_0(\Prefix, \x, \y). \nn
\end{align}
