# Supplementary material for: Optimal Sparse Decision Trees
Source: arXiv:1904.12847 source file (2023-09-26)
Supplement: Supplementary file 2 [file appendix.tex]

\clearpage
\section{Data Processing Details and Antecedent Mining}
\label{appendix:data}

In this appendix, we provide details regarding datasets used in our experiments
(Section~\ref{sec:experiments}).

\subsection{ProPublica Recidivism Data Set}
The original dataset contains 7,214 records; we keep the 6,907 records
containing a `c\_jail\_in' date.
To compute an individual's age, we subtract the value in the `dob' field from
that in the `c\_jail\_in' field.

Table~\ref{tab:recidivism-data} shows the~6 attributes
and corresponding~17 categorical values
that we use for the ProPublica data set.
From these, we construct~17 single-clause antecedents, for example,
${(age = 23-25)}$.
We then combine pairs of these antecedents as conjunctions to form
two-clause antecedents, \eg ${(age = 23-25) \wedge (priors = 2-3)}$.
By virtue of our lower bound on antecedent support,
(Theorem~\ref{thm:min-capture},~\S\ref{sec:lb-support}),
we eliminate antecedents with support less than~0.005 or greater than~0.995,
since ${\Reg = 0.005}$ is the smallest regularization parameter value
we study for this problem.
With this filtering step, we generate between~121 and~123 antecedents for each fold;
without it, we would instead generate about~130 antecedents as input to our algorithm.

Note that we exclude the `current charge' attribute (which has two categorical values,
`misdemeanor' and `felony'); for individuals in the data set booked on multiple charges,
this attribute does not appear to consistently reflect the most serious charge.

\begin{table}[h!]
\centering
%$Q_\text{max}$ $K_\text{max}$
\begin{tabular}{l  | c  c  c}
Feature & Value range & Categorical values & Count \\
\hline
sex & --- & male, female & 2 \\
age & 18-96 & 18-20, 21-22, 23-25, 26-45, $>$45  & 5 \\
juvenile felonies & 0-20 & 0, $>$0 & 2 \\
juvenile misdemeanors & 0-13 & 0, $>$0 & 2 \\
%other juvenile crimes & 0-17 & --- & 2 \\
juvenile crimes & 0-21 & 0, $>$0 & 2 \\
priors & 0-38 & 0, 1, 2-3, $>$3 & 4
\end{tabular}
%\vspace{4mm}
\caption{Categorical features (6 attributes, 17 values) from the ProPublica data set.
We construct the feature \emph{juvenile crimes} from the sum of
\emph{juvenile felonies}, \emph{juvenile misdemeanors}, and
the number of juvenile crimes that were neither felonies nor misdemeanors (not shown).
}
\vspace{4mm}
\label{tab:recidivism-data}
\end{table}

\subsection{NYPD Stop-and-frisk Data Set}
This data set is larger than, but similar to the NYCLU stop-and-frisk data set, 
described next.

%\newpage
\subsection{NYCLU Stop-and-frisk Data Set}
The original data set contains 45,787 records,
each describing an incident involving a stopped person; the individual
was frisked in 30,345 (66.3\%) of records and and searched in 7,283 (15.9\%).
In 30,961 records, the individual was frisked and/or searched (67.6\%); of those,
a criminal possession of a weapon was identified 1,445 times (4.7\% of these records).
We remove 1,929 records with missing data, as well as a small number with extreme values
for the individual's age---we eliminate those with age~${< 12}$ or~${>89}$.
%we also assume that one age marked `366' is a typo, and we replace it with `36'.
%
This yields a set of 29,595 records in which the individual was frisked and/or searched.
To address the class imbalance for this problem, we sample records from the
smaller class with replacement.
We generate cross-validation folds first, and then resample within each fold.
In our 10-fold cross-validation experiments, each training set contains 50,743 observations.
Table~\ref{tab:frisk-data} shows the 5 categorical attributes that we use,
corresponding to a total of 28 values.
Our experiments use these antecedents,
as well as negations of the 18 antecedents corresponding to the two features
\emph{stop reason} and \emph{additional circumstances},
which gives a total of 46 antecedents.

\begin{table}[h!]
\centering
%$Q_\text{max}$ $K_\text{max}$
\begin{tabular}{l | c  c}
Feature & Values & Count \\
\hline
stop reason & suspicious object, fits description, casing, & 9 \\
& acting as lookout, suspicious clothing, & \\
& drug transaction, furtive movements, & \\
& actions of violent crime, suspicious bulge \\
\hline
additional & proximity to crime scene, evasive response,  & 9 \\
circumstances & associating with criminals, changed direction, & \\
& high crime area, time of day,  & \\
& sights and sounds of criminal activity, & \\
& witness report, ongoing investigation & \\
\hline
city & Queens,  Manhattan, Brooklyn, Staten Island, Bronx & 5 \\
\hline
location & housing authority, transit authority, & 3 \\
& neither housing nor transit authority & \\
\hline
inside or outside & inside, outside & 2 \\
\end{tabular}
%\vspace{4mm}
\caption{Categorical features (5 attributes, 28 values) from the NYCLU data set.}
\vspace{4mm}
\label{tab:frisk-data}
\end{table}

%\clearpage
\section{Example Optimal Rule Lists, for Different Values of~$\Reg$}
\label{appendix:examples}

For each of our prediction problems, we provide listings of
optimal rule lists found by CORELS, across 10 cross-validation folds,
for different values of the regularization parameter~$\Reg$.
These rule lists correspond to the results for CORELS summarized
in Figures~\ref{fig:sparsity-compas} and~\ref{fig:sparsity-weapon}~(\S\ref{sec:sparsity}).
Recall that as~$\Reg$ decreases, optimal rule lists tend to grow in length. \\

\subsection{ProPublica Recidivism Data Set}
We show example optimal rule lists that predict two-year recidivism.
Figure~\ref{fig:recidivism-rule-list-02-01} shows examples for
regularization parameters~${\Reg = 0.02}$ and~0.01.
Figure~\ref{fig:recidivism-rule-list-005} shows examples for~${\Reg = 0.005}$;
Figure~\ref{fig:recidivism-all-folds}~(\S\ref{sec:examples}) showed two representative examples.

For the largest regularization parameter~${\Reg = 0.02}$~(Figure~\ref{fig:recidivism-rule-list-02-01}),
we observe that all folds identify the same length-1 rule list.
For the intermediate value~${\Reg = 0.01}$ (Figure~\ref{fig:recidivism-rule-list-02-01}),
the folds identify optimal 2-rule or 3-rule lists that contain the nearly same prefix rules,
up to permutations.
For the smallest value~${\Reg = 0.005}$~(Figure~\ref{fig:recidivism-rule-list-005}),
the folds identify optimal 3-rule or 4-rule lists that contain the nearly same prefix rules,
up to permutations.
Across all three regularization parameter values and all folds,
the prefix rules always predict the positive class label,
and the default rule always predicts the negative class label.
We note that our objective is not designed to enforce any of these properties.
%though some may be seen as desirable.

% tail -n 1 ../logs/for-compas_*_train.out-curious_lb-with_prefix_perm_map-minor-removed=none-max_num_nodes=10000000-c=0.0200000-v=progress-f=1000-opt.txt
%{priors:>3}~1;default~0
%
%$ tail -n 1 ../logs/for-compas_*_train.out-curious_lb-with_prefix_perm_map-minor-removed=none-max_num_nodes=10000000-c=0.0100000-v=progress-f=1000-opt.txt
%{priors:>3}~1;{sex:Male,juvenile-crimes:>0}~1;default~0 x 3
%{sex:Male,juvenile-crimes:>0}~1;{priors:>3}~1;default~0 x 2
%{sex:Male,age:18-20}~1;{priors:>3}~1;default~0 x 2
%{age:21-22,priors:2-3}~1;{priors:>3}~1;{sex:Male,age:18-20}~1;default~0 x 2
%{priors:>3}~1;{sex:Male,age:18-20}~1;default~0
\begin{figure}[h!]
\textbf{Two-year recidivism prediction $(\Reg = 0.02)$}
\vspace{1mm}
\begin{algorithmic}
\State \bif $(priors > 3)$ \bthen $yes$ \Comment{Found by all 10 folds}
\State \belse $no$
\end{algorithmic}
\vspace{5mm}
\textbf{Two-year recidivism prediction $(\Reg = 0.01)$}
\vspace{1mm}
\begin{algorithmic}
\State \bif $(priors > 3)$ \bthen $yes$ \Comment{Found by 3 folds}
\State \belif $(sex = male) \band (juvenile~crimes > 0)$ \bthen $yes$
\State \belse $no$
\end{algorithmic}
\vspace{1mm}
\begin{algorithmic}
\State \bif $(sex = male) \band (juvenile~crimes > 0)$ \bthen $yes$ \Comment{Found by 2 folds}
\State \belif $(priors > 3)$ \bthen $yes$
\State \belse $no$
\end{algorithmic}
\vspace{1mm}
\begin{algorithmic}
\State \bif $(age = 21-22) \band (priors = 2-3)$ \bthen $yes$ \Comment{Found by 2 folds}
\State \belif $(priors > 3)$ \bthen $yes$
\State \belif $(age = 18-20) \band (sex = male)$ \bthen $yes$
\State \belse $no$
\end{algorithmic}
\vspace{1mm}
\begin{algorithmic}
\State \bif $(age = 18-20) \band (sex = male)$ \bthen $yes$ \Comment{Found by 2 folds}
\State \belif $(priors > 3)$ \bthen $yes$
\State \belse $no$
\end{algorithmic}
\vspace{1mm}
\begin{algorithmic}
\State \bif $(priors > 3)$ \bthen $yes$ \Comment{Found by 1 fold}
\State \belif $(age = 18-20) \band (sex = male)$ \bthen $yes$
\State \belse $no$
\end{algorithmic}
\caption{Example optimal rule lists for the ProPublica data set,
found by CORELS with regularization parameters~${\Reg = 0.02}$~(top),
and~0.01~(bottom) across 10 cross-validation folds.
}
\label{fig:recidivism-rule-list-02-01}
\end{figure}

%logs in jmlr/ from Nicholas 9/27
%$ tail -n 1 *compas*curious*with*-minor*none-m*1000000000*0.005*opt.txt
%{sex:Male,age:18-20}~1;{age:21-22,priors:2-3}~1;{priors:>3}~1;default~0 x 4
%{age:21-22,priors:2-3}~1;{priors:>3}~1;{sex:Male,age:18-20}~1;default~0 x 2
%{sex:Male,age:18-20}~1;{priors:>3}~1;{age:21-22,priors:2-3}~1;default~0
%{sex:Male,age:18-20}~1;{age:21-22,priors:2-3}~1;{age:23-25,priors:2-3}~1;{priors:>3}~1;default~0
%{sex:Male,age:18-20}~1;{age:21-22,priors:2-3}~1;{priors:>3}~1;{age:23-25,priors:2-3}~1;default~0
%{age:21-22,priors:2-3}~1;{age:23-25,priors:2-3}~1;{priors:>3}~1;{sex:Male,age:18-20}~1;default~0
\begin{figure}[h!]
\textbf{Two-year recidivism prediction $(\Reg = 0.005)$}
\vspace{1mm}
\begin{algorithmic}
\State \bif $(age = 18-20) \band (sex = male)$ \bthen $yes$ \Comment{Found by 4 folds}
\State \belif $(age = 21-22) \band (priors = 2-3)$ \bthen $yes$
\State \belif $(priors > 3)$ \bthen $yes$
\State \belse $no$
\end{algorithmic}
\vspace{1mm}
\begin{algorithmic}
\State \bif $(age = 21-22) \band (priors = 2-3)$ \bthen $yes$  \Comment{Found by 2 folds}
\State \belif $(priors > 3)$ \bthen $yes$
\State \belif $(age = 18-20) \band (sex = male)$ \bthen $yes$
\State \belse $no$
\end{algorithmic}
\vspace{1mm}
\begin{algorithmic}
\State \bif $(age = 18-20) \band (sex = male)$ \bthen $yes$ \Comment{Found by 1 fold}
\State \belif $(priors > 3)$ \bthen $yes$
\State \belif $(age = 21-22) \band (priors = 2-3)$ \bthen $yes$
\State \belse $no$
\end{algorithmic}
\vspace{1mm}
\begin{algorithmic}
\State \bif $(age = 18-20) \band (sex = male)$ \bthen $yes$ \Comment{Found by 1 fold}
\State \belif $(age = 21-22) \band (priors = 2-3)$ \bthen $yes$
\State \belif $(age = 23-25) \band (priors = 2-3)$ \bthen $yes$
\State \belif $(priors > 3)$ \bthen $yes$
\State \belse $no$
\end{algorithmic}
\vspace{1mm}
\begin{algorithmic}
\State \bif $(age = 18-20) \band (sex = male)$ \bthen $yes$ \Comment{Found by 1 fold}
\State \belif $(age = 21-22) \band (priors = 2-3)$ \bthen $yes$
\State \belif $(priors > 3)$ \bthen $yes$
\State \belif $(age = 23-25) \band (priors = 2-3)$ \bthen $yes$
\State \belse $no$
\end{algorithmic}
\vspace{1mm}
\begin{algorithmic}
\State \bif $(age = 21-22) \band (priors = 2-3)$ \bthen $yes$ \Comment{Found by 1 fold}
\State \belif $(age = 23-25) \band (priors = 2-3)$ \bthen $yes$
\State \belif $(priors > 3)$ \bthen $yes$
\State \belif $(age = 18-20) \band (sex = male)$ \bthen $yes$
\State \belse $no$
\end{algorithmic}
\caption{Example optimal rule lists for the ProPublica data set,
found by CORELS with regularization parameters~${\Reg = 0.005}$,
across 10 cross-validation folds.
}
\label{fig:recidivism-rule-list-005}
\end{figure}

\clearpage
\subsection{NYPD Stop-and-frisk Data Set}
We show example optimal rule lists that predict whether a weapon
will be found on a stopped individual who is frisked or searched, learned from the NYPD data set.

\begin{figure}[b!]
%$ head *cpw_*0.01*opt* K = 2
%{cs_objcs:stop-reason=suspicious-object}~1;{location:transit-authority}~1;default~0 x 8
%{location:transit-authority}~1;{cs_objcs:stop-reason=suspicious-object}~1;default~0 x 2
\textbf{Weapon prediction $(\Reg = 0.01, \text{Feature Set~C})$}
\vspace{1mm}
\begin{algorithmic}
\State \bif $(stop~reason = suspicious~object)$ \bthen $yes$ \Comment{Found by 8 folds}
\State \belif $(location = transit~authority)$ \bthen $yes$
\State \belse $no$
\end{algorithmic}
\vspace{1mm}
\begin{algorithmic}
\State \bif $(location = transit~authority)$ \bthen $yes$ \Comment{Found by 2 folds}
\State \belif $(stop~reason = suspicious~object)$ \bthen $yes$
\State \belse $no$
\end{algorithmic}
\vspace{5mm}
%$ head *cpw_*0.005*opt* K = 4 or 5
%{cs_objcs:stop-reason=suspicious-object}~1;{location:transit-authority}~1;{location:housing-authority}~0;{city:MANHATTAN}~1;default~0 x 7
%{cs_objcs:stop-reason=suspicious-object}~1;{location:housing-authority}~0;{location:transit-authority}~1;{city:MANHATTAN}~1;default~0
%{cs_objcs:stop-reason=suspicious-object}~1;{location:housing-authority}~0;{city:MANHATTAN}~1;{location:transit-authority}~1;default~0
%{cs_objcs:stop-reason=suspicious-object}~1;{location:transit-authority}~1;{city:BRONX}~0;{location:housing-authority}~0;{cs_furtv:stop-reason=furtive-movements}~0;default~1
\textbf{Weapon prediction $(\Reg = 0.005, \text{Feature Set~C})$}
\begin{algorithmic}
\State \bif $(stop~reason = suspicious~object)$ \bthen $yes$ \Comment{Found by 7 folds}
\State \belif $(location = transit~authority)$ \bthen $yes$
\State \belif $(location = housing~authority)$ \bthen $no$
\State \belif $(city = Manhattan)$ \bthen $yes$
\State \belse $no$
\end{algorithmic}
\vspace{1mm}
\begin{algorithmic}
\State \bif $(stop~reason = suspicious~object)$ \bthen $yes$ \Comment{Found by 1 fold}
\State \belif $(location = housing~authority)$ \bthen $no$
\State \belif $(location = transit~authority)$ \bthen $yes$
\State \belif $(city = Manhattan)$ \bthen $yes$
\State \belse $no$
\end{algorithmic}
\vspace{1mm}
\begin{algorithmic}
\State \bif $(stop~reason = suspicious~object)$ \bthen $yes$ \Comment{Found by 1 fold}
\State \belif $(location = housing~authority)$ \bthen $no$
\State \belif $(city = Manhattan)$ \bthen $yes$
\State \belif $(location = transit~authority)$ \bthen $yes$
\State \belse $no$
\end{algorithmic}
\vspace{1mm}
\begin{algorithmic}
\State \bif $(stop~reason = suspicious~object)$ \bthen $yes$ \Comment{Found by 1 fold}
\State \belif $(location = transit~authority)$ \bthen $yes$
\State \belif $(city = Bronx)$ \bthen $no$
\State \belif $(location = housing~authority)$ \bthen $no$
\State \belif $(stop~reason = furtive~movements)$ \bthen $no$
\State \belse $yes$
\end{algorithmic}
\caption{Example optimal rule lists for the NYPD stop-and-frisk data set,
found by CORELS with regularization parameters~${\Reg = 0.01}$~(top) and~0.005~(bottom),
across 10 cross-validation folds.
}
\label{fig:cpw-rule-list}
\end{figure}

\begin{figure}[b!]
%$ head *cpw-noloc_*0.01*opt* K = 2
%{cs_objcs:stop-reason=suspicious-object}~1;{inout:outside}~0;default~1 x 7
%{cs_objcs:stop-reason=suspicious-object}~1;{inout:inside}~1;default~0 x 3
\textbf{Weapon prediction $(\Reg = 0.01, \text{Feature Set~D})$}
\vspace{1mm}
\begin{algorithmic}
\State \bif $(stop~reason = suspicious~object)$ \bthen $yes$ \Comment{Found by 7 folds}
\State \belif $(inside~or~outside = outside)$ \bthen $no$
\State \belse $yes$
\end{algorithmic}
\vspace{1mm}
\begin{algorithmic}
\State \bif $(stop~reason = suspicious~object)$ \bthen $yes$ \Comment{Found by 3 folds}
\State \belif $(inside~or~outside = inside)$ \bthen $yes$
\State \belse $no$
\end{algorithmic}
\vspace{5mm}
%$ head *cpw-noloc_*0.005*opt* K = 4
%{cs_objcs:stop-reason=suspicious-object}~1;{cs_lkout:stop-reason=acting-as-lookout}~0;{cs_descr:stop-reason=fits-description}~0;{cs_furtv:stop-reason=furtive-movements}~0;default~1 x 2
%{cs_objcs:stop-reason=suspicious-object}~1;{cs_furtv:stop-reason=furtive-movements}~0;{cs_lkout:stop-reason=acting-as-lookout}~0;{cs_descr:stop-reason=fits-description}~0;default~1 x 2
%{cs_objcs:stop-reason=suspicious-object}~1;{cs_lkout:stop-reason=acting-as-lookout}~0;{cs_furtv:stop-reason=furtive-movements}~0;{cs_descr:stop-reason=fits-description}~0;default~1
%{cs_objcs:stop-reason=suspicious-object}~1;{cs_descr:stop-reason=fits-description}~0;{cs_lkout:stop-reason=acting-as-lookout}~0;{cs_furtv:stop-reason=furtive-movements}~0;default~1
%{cs_objcs:stop-reason=suspicious-object}~1;{cs_furtv:stop-reason=furtive-movements}~0;{cs_descr:stop-reason=fits-description}~0;{cs_lkout:stop-reason=acting-as-lookout}~0;default~1
%
%{cs_objcs:stop-reason=suspicious-object}~1;{cs_descr:stop-reason=fits-description}~0;{cs_casng:stop-reason=casing}~0;{cs_furtv:stop-reason=furtive-movements}~0;default~1
%{cs_objcs:stop-reason=suspicious-object}~1;{cs_casng:stop-reason=casing}~0;{cs_descr:stop-reason=fits-description}~0;{cs_furtv:stop-reason=furtive-movements}~0;default~1
%{cs_objcs:stop-reason=suspicious-object}~1;{cs_casng:stop-reason=casing}~0;{cs_furtv:stop-reason=furtive-movements}~0;{cs_descr:stop-reason=fits-description}~0;default~1
\textbf{Weapon prediction $(\Reg = 0.005, \text{Feature Set~D})$}
\vspace{1mm}
\begin{algorithmic}
\State \bif $(stop~reason = suspicious~object)$ \bthen $yes$ \Comment{Found by 2 folds}
\State \belif $(stop~reason = acting~as~lookout)$ \bthen $no$
\State \belif $(stop~reason = fits~description)$ \bthen $no$
\State \belif $(stop~reason = furtive~movements)$ \bthen $no$
\State \belse $yes$
\end{algorithmic}
\vspace{1mm}
\begin{algorithmic}
\State \bif $(stop~reason = suspicious~object)$ \bthen $yes$ \Comment{Found by 2 folds}
\State \belif $(stop~reason = furtive~movements)$ \bthen $no$
\State \belif $(stop~reason = acting~as~lookout)$ \bthen $no$
\State \belif $(stop~reason = fits~description)$ \bthen $no$
\State \belse $yes$
\end{algorithmic}
\vspace{1mm}
\begin{algorithmic}
\State \bif $(stop~reason = suspicious~object)$ \bthen $yes$ \Comment{Found by 1 fold}
\State \belif $(stop~reason = acting~as~lookout)$ \bthen $no$
\State \belif $(stop~reason = furtive~movements)$ \bthen $no$
\State \belif $(stop~reason = fits~description)$ \bthen $no$
\State \belse $yes$
\end{algorithmic}
\begin{algorithmic}
\vspace{1mm}
\State \bif $(stop~reason = suspicious~object)$ \bthen $yes$ \Comment{Found by 1 fold}
\State \belif $(stop~reason = fits~description)$ \bthen $no$
\State \belif $(stop~reason = acting~as~lookout)$ \bthen $no$
\State \belif $(stop~reason = furtive~movements)$ \bthen $no$
\State \belse $yes$
\end{algorithmic}
\vspace{1mm}
\begin{algorithmic}
\State \bif $(stop~reason = suspicious~object)$ \bthen $yes$ \Comment{Found by 1 fold}
\State \belif $(stop~reason = furtive~movements)$ \bthen $no$
\State \belif $(stop~reason = fits~description)$ \bthen $no$
\State \belif $(stop~reason = acting~as~lookout)$ \bthen $no$
\State \belse $yes$
\end{algorithmic}
\caption{Example optimal rule lists for the NYPD stop-and-frisk data set (Feature Set~D)
found by CORELS with regularization parameters~${\Reg = 0.01}$~(top) and~0.005~(bottom),
across 10 cross-validation folds.
For~${\Reg = 0.005}$, we show results from~7 folds; the remaining~3 folds were equivalent,
up to a permutation of the prefix rules, and started with the same first prefix rule.
}
\label{fig:cpw-noloc-rule-list}
\end{figure}

\clearpage
\subsection{NYCLU Stop-and-frisk Data Set}
We show example optimal rule lists that predict whether a weapon
will be found on a stopped individual who is frisked or searched, learned from the NYCLU data set.
Figure~\ref{fig:weapon-rule-list-04-01} shows
regularization parameters~${\Reg = 0.04}$ and~0.01,
and Figure~\ref{fig:weapon-rule-list-0025} shows~${\Reg = 0.0025}$.
We showed a representative solution for~${\Reg = 0.01}$ in
Figure~\ref{fig:weapon-rule-list}~(\S\ref{sec:examples}).

For each of the two larger regularization parameters in Figure~\ref{fig:weapon-rule-list-04-01},
${\Reg = 0.04}$~(top) and 0.01~(bottom), we observe that across the folds,
all the optimal rule lists contain the same or equivalent rules, up to a permutation.
With the smaller regularization parameter~${\Reg = 0.0025}$ (Figure~\ref{fig:weapon-rule-list-0025}),
we observe a greater diversity of longer optimal rule lists, though they share similar structure.

%logs in jmlr/ from Nicholas 9/27
%tail -n 1 tail -n 1 *weapon*0.04*opt.txt
%{cs_objcs:stop-reason=suspicious-object}~1;{cs_bulge:stop-reason=not-suspicious-bulge}~0;default~1 x 7
%{cs_bulge:stop-reason=suspicious-bulge}~1;{cs_objcs:stop-reason=not-suspicious-object}~0;default~1 x 3
%
%$ tail -n 1 *weapon*curious*with*-minor-*none*1000000000*0.01*opt.txt
%{cs_objcs:stop-reason=suspicious-object}~1;{location:transit-authority}~1;{cs_bulge:stop-reason=not-suspicious-bulge}~0;default~1 x 4
%{location:transit-authority}~1;{cs_bulge:stop-reason=suspicious-bulge}~1;{cs_objcs:stop-reason=suspicious-object}~1;default~0 x 3
%{location:transit-authority}~1;{cs_objcs:stop-reason=suspicious-object}~1;{cs_bulge:stop-reason=suspicious-bulge}~1;default~0 x 2
%{location:transit-authority}~1;{cs_objcs:stop-reason=suspicious-object}~1;{cs_bulge:stop-reason=not-suspicious-bulge}~0;default~1
\begin{figure}[b!]
\textbf{Weapon prediction $(\Reg = 0.04)$}
\vspace{1mm}
\begin{algorithmic}
\State \bif $(stop~reason = suspicious~object)$ \bthen $yes$ \Comment{Found by 7 folds}
\State \belif $(stop~reason \neq suspicious~bulge)$ \bthen $no$
\State \belse $yes$
\end{algorithmic}
\vspace{1mm}
\begin{algorithmic}
\State \bif $(stop~reason = suspicious~bulge)$ \bthen $yes$ \Comment{Found by 3 folds}
\State \belif $(stop~reason \neq suspicious~object)$ \bthen $no$
\State \belse $yes$
\end{algorithmic}
\vspace{5mm}
\textbf{Weapon prediction $(\Reg = 0.01)$}
\vspace{1mm}
\begin{algorithmic}
\State \bif $(stop~reason = suspicious~object)$ \bthen $yes$ \Comment{Found by 4 folds}
\State \belif $(location = transit~authority)$ \bthen $yes$
\State \belif $(stop~reason \neq suspicious~bulge)$ \bthen $no$
\State \belse $yes$
\end{algorithmic}
\vspace{1mm}
\begin{algorithmic}
\State \bif $(location = transit~authority)$ \bthen $yes$ \Comment{Found by 3 folds}
\State \belif $(stop~reason = suspicious~bulge)$ \bthen $yes$
\State \belif $(stop~reason = suspicious~object)$ \bthen $yes$
\State \belse $no$
\end{algorithmic}
\vspace{1mm}
\begin{algorithmic}
\State \bif $(location = transit~authority)$ \bthen $yes$ \Comment{Found by 2 folds}
\State \belif $(stop~reason = suspicious~object)$ \bthen $yes$
\State \belif $(stop~reason = suspicious~bulge)$ \bthen $yes$
\State \belse $no$
\end{algorithmic}
\vspace{1mm}
\begin{algorithmic}
\State \bif $(location = transit~authority)$ \bthen $yes$ \Comment{Found by 1 fold}
\State \belif $(stop~reason = suspicious~object)$ \bthen $yes$
\State \belif $(stop~reason \neq suspicious~bulge)$ \bthen $no$
\State \belse $yes$
\end{algorithmic}
\caption{Example optimal rule lists for the NYCLU stop-and-frisk data set,
found by CORELS with regularization parameters~${\Reg = 0.04}$~(top) and~0.01~(bottom),
across 10 cross-validation folds.
}
\label{fig:weapon-rule-list-04-01}
\end{figure}

\begin{figure}[h!]
\textbf{Weapon prediction $(\Reg = 0.0025)$}
\vspace{0.5mm}
\scriptsize
\begin{algorithmic}
\State \bif $(stop~reason = suspicious~object)$ \bthen $yes$ \Comment{Found by 4 folds $(K=7)$}
\State \belif $(stop~reason = casing)$ \bthen $no$
\State \belif $(stop~reason = suspicious~bulge)$ \bthen $yes$
\State \belif $(stop~reason = fits~description)$ \bthen $no$
\State \belif $(location = transit~authority)$ \bthen $yes$
\State \belif $(inside~or~outside = inside)$ \bthen $no$
\State \belif $(city = Manhattan)$ \bthen $yes$
\State \belse $no$
\end{algorithmic}
\vspace{0.5mm}
\begin{algorithmic}
\State \bif $(stop~reason = suspicious~object)$ \bthen $yes$ \Comment{Found by 1 fold $(K=6)$}
\State \belif $(stop~reason = casing)$ \bthen $no$
\State \belif $(stop~reason = suspicious~bulge)$ \bthen $yes$
\State \belif $(stop~reason = fits~description)$ \bthen $no$
\State \belif $(location = housing~authority)$ \bthen $no$
\State \belif $(city = Manhattan)$ \bthen $yes$
\State \belse $no$
\end{algorithmic}
\vspace{0.5mm}
\begin{algorithmic}
\State \bif $(stop~reason = suspicious~object)$ \bthen $yes$ \Comment{Found by 1 fold $(K=6)$}
\State \belif $(stop~reason = suspicious~bulge)$ \bthen $yes$
\State \belif $(location = housing~authority)$ \bthen $no$
\State \belif $(stop~reason = casing)$ \bthen $no$
\State \belif $(stop~reason = fits~description)$ \bthen $no$
\State \belif $(city = Manhattan)$ \bthen $yes$
\State \belse $no$
\end{algorithmic}
\vspace{0.5mm}
\begin{algorithmic}
\State \bif $(stop~reason = suspicious~object)$ \bthen $yes$ \Comment{Found by 1 fold $(K=6)$}
\State \belif $(stop~reason = casing)$ \bthen $no$
\State \belif $(stop~reason = suspicious~bulge)$ \bthen $yes$
\State \belif $(stop~reason = fits~description)$ \bthen $no$
\State \belif $(location = housing~authority)$ \bthen $no$
\State \belif $(city = Manhattan)$ \bthen $yes$
\State \belse $no$
\end{algorithmic}
\vspace{0.5mm}
\begin{algorithmic}
\State \bif $(stop~reason = drug~transaction)$ \bthen $no$ \Comment{Found by 1 fold $(K=8)$}
\State \belif $(stop~reason = suspicious~object)$ \bthen $yes$
\State \belif $(stop~reason = suspicious~bulge)$ \bthen $yes$
\State \belif $(location = housing~authority)$ \bthen $no$
\State \belif $(stop~reason = fits~description)$ \bthen $no$
\State \belif $(stop~reason = casing)$ \bthen $no$
\State \belif $(city = Manhattan)$ \bthen $yes$
\State \belif $(city = Bronx)$ \bthen $yes$
\State \belse $no$
\end{algorithmic}
\vspace{0.5mm}
\begin{algorithmic}
\State \bif $(stop~reason = suspicious~object)$ \bthen $yes$ \Comment{Found by 1 fold $(K=9)$}
\State \belif $(stop~reason = casing)$ \bthen $no$
\State \belif $(stop~reason = suspicious~bulge)$ \bthen $yes$
\State \belif $(stop~reason = fits~description)$ \bthen $no$
\State \belif $(location = transit~authority)$ \bthen $yes$
\State \belif $(inside~or~outside = inside)$ \bthen $no$
\State \belif $(city = Manhattan)$ \bthen $yes$
\State \belif $(additional~circumstances = changed~direction)$ \bthen $no$
\State \belif $(city = Bronx)$ \bthen $yes$
\State \belse $no$
\end{algorithmic}
\vspace{0.5mm}
%{cs_objcs:stop-reason=suspicious-object}~1;{cs_casng:stop-reason=casing}~0;{cs_bulge:stop-reason=suspicious-bulge}~1;{cs_vcrim:stop-reason=actions-of-violent-crime}~0;{cs_descr:stop-reason=fits-description}~0;{location:transit-authority}~1;{inout:inside}~0;{city:Manhattan}~1;{ac_evasv:circumstances=evasive-response}~0;{city:Bronx}~1;default~0
\begin{algorithmic}
\State \bif $(stop~reason = suspicious~object)$ \bthen $yes$ \Comment{Found by 1 fold $(K=10)$}
\State \belif $(stop~reason = casing)$ \bthen $no$
\State \belif $(stop~reason = suspicious~bulge)$ \bthen $yes$
\State \belif $(stop~reason = actions~of~violent~crime)$ \bthen $no$
\State \belif $(stop~reason = fits~description)$ \bthen $no$
\State \belif $(location = transit~authority)$ \bthen $yes$
\State \belif $(inside~or~outside = inside)$ \bthen $no$
\State \belif $(city = Manhattan)$ \bthen $yes$
\State \belif $(additional~circumstances = evasive~response)$ \bthen $no$
\State \belif $(city = Bronx)$ \bthen $yes$
\State \belse $no$
\end{algorithmic}
\caption{Example optimal rule lists for the NYCLU stop-and-frisk data set~${\Reg = 0.0025}$.
%found by CORELS with regularization parameter, across 10 cross-validation folds.
}
\label{fig:weapon-rule-list-0025}
\end{figure}

\clearpage
\section{Additional Results on Predictive Performance and Model Size for
CORELS and Other Algorithms}
\label{appendix:cpw}

In this appendix, we plot TPR, FPR, and model size for CORELS and three other
algorithms, using the NYPD data set (Feature Set~D).

\begin{figure}[htb!]
\begin{center}
%\includegraphics[width=0.75\textwidth]{figs/sketch-comparison.png}
% left lower right upper
\includegraphics[trim={17mm, 0mm, 27mm, 0mm},
width=0.7\textwidth]{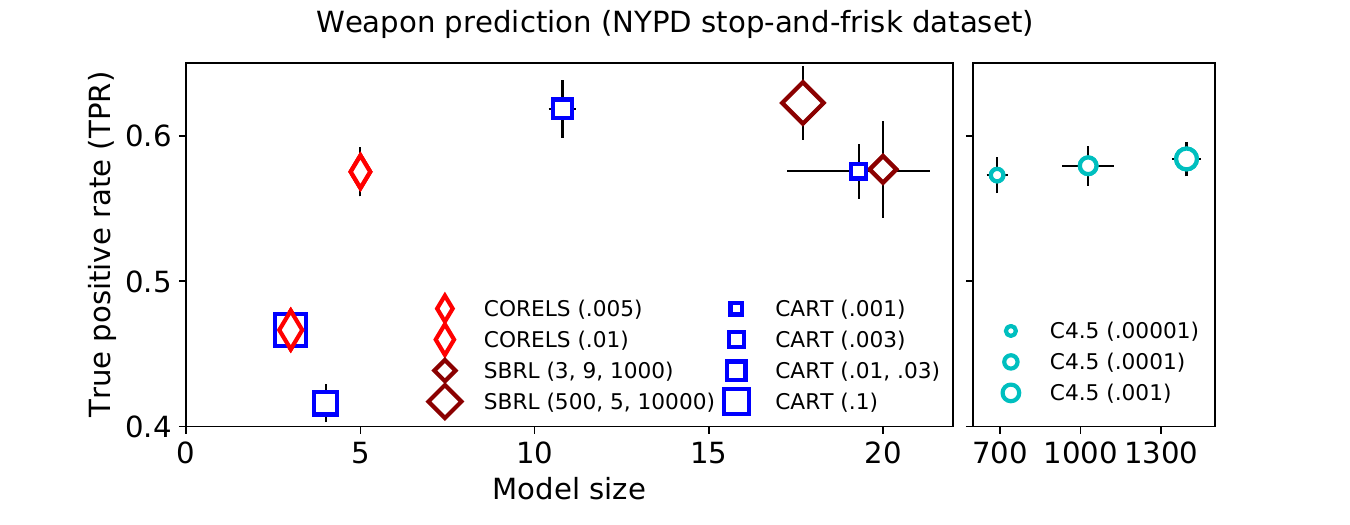}
\includegraphics[trim={17mm, 10mm, 27mm, 4mm},
width=0.7\textwidth]{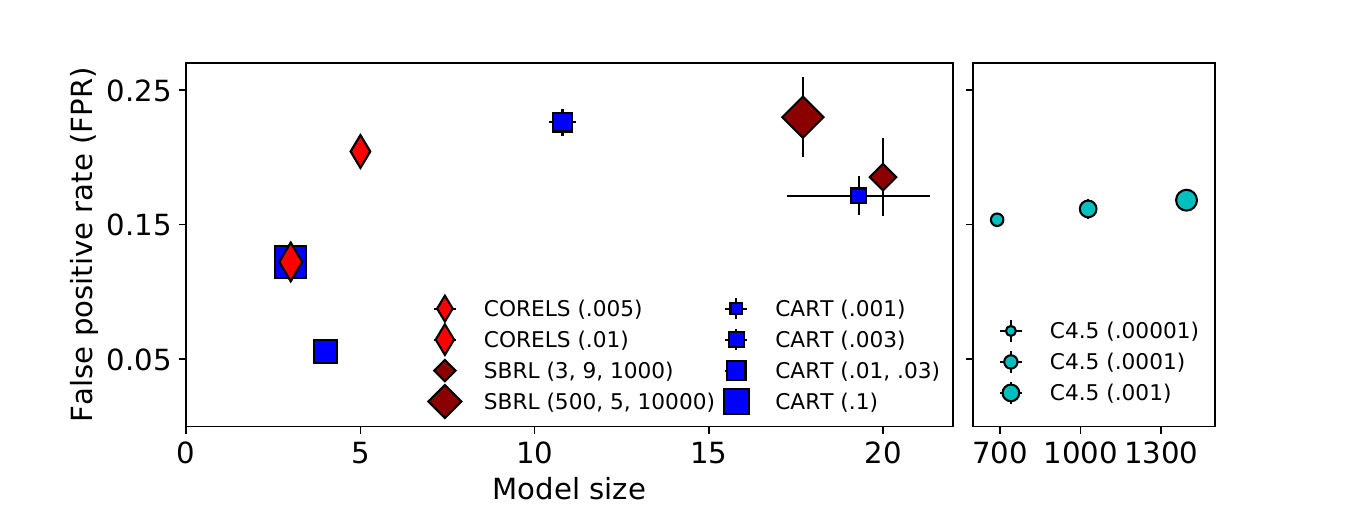}
\end{center}
\caption{TPR (top) and FPR (bottom)
for the test set, as a function of model size, across different methods,
for weapon prediction with the NYPD stop-and-frisk data set (Feature Set~D).
In the legend, numbers in parentheses are algorithm parameters,
as in Figure~\ref{fig:sparsity-weapon}.
Legend markers and error bars indicate means and standard deviations,
respectively, across cross-validation folds.
%
%For CORELS and SBRL, we use ${M = 28}$ antecedents.
%
%CART with ${cp = 0.001}$ significantly overfits;
%C4.5 finds large models and dramatically overfits for all tested parameters.
C4.5 finds large models for all tested parameters.
}
\label{fig:sparsity-cpw}
\end{figure}
